# Supplementary material for: Towards Aligning Language Models with Textual Feedback
Source: arXiv:2407.16970 source file (2025-03-18)
Supplement: Supplementary file 1 [file hh_steerability.tex]

We conducted a small evaluation setting to assess the steerability of our model at run-time. To do so, we evaluated our last model checkpoint when conditioned on \texttt{Harmful} instead of \texttt{Harmless and very helpful}. We notice that this leads to generations being slightly less \texttt{Harmless and very helpful} (65.1 $\rightarrow$ 60.0) and slightly more \texttt{Harmful} (11.6 $\rightarrow$ 15.1), but that our model is not steerable at inference time to produce harmful content. This is consistent with our exploitation of the exemplar feedback commented in \ref{subsec:exemplar_feedback}. Similarly to PPO and DPO, by using a single exemplar feedback, we are steering our model towards an implicit set of user preferences, i.e., being harmless and very helpful, and thus our model struggles when asked to elicit the opposite behavior.
